# Supplementary material for: Rayleigh-B\'enard convection of a model emulsion: anomalous heat-flux fluctuations and finite-size droplets effects
Source: arXiv:2101.03374 ancillary file (2021-02-19)
Supplement: Supplementary file 1 [file esi.pdf]

# Electronic Supplementary Information for "Rayleigh-Bénard convection of a model emulsion: anomalous heat-flux fluctuations and finite-size droplets effects"

**Francesca Pelusi***
Department of Physics & INFN, University of Rome "Tor Vergata"
Via della Ricerca Scientifica 1, 00133 Rome, Italy
f.pelusi@fz-juelich.de

**Mauro Sbragaglia**
Department of Physics & INFN, University of Rome "Tor Vergata"
Via della Ricerca Scientifica 1, 00133 Rome, Italy

**Roberto Benzi**
Department of Physics & INFN, University of Rome "Tor Vergata"
Via della Ricerca Scientifica 1, 00133 Rome, Italy

**Andrea Scagliarini**
Istituto per le Applicazioni del Calcolo, CNR
Via dei Taurini 19, 00185 Rome, Italy

**Massimo Bernaschi**
Istituto per le Applicazioni del Calcolo, CNR
Via dei Taurini 19, 00185 Rome, Italy

**Sauro Succi**
Istituto per le Applicazioni del Calcolo, CNR
Via dei Taurini 19, 00185 Rome, Italy
Center for Life Nano Science Sapienza, Istituto Italiano di Tecnologia
Viale Regina Elena 295, 00161 Rome, Italy

*Current affiliation: Forschungszentrum Jülich GmbH, Helmholtz Institute Erlangen-Nürnberg for Renewable Energy (IEK-11) - Cauerstraße 1, 91052 Erlangen, Germany

# 1 Supplementary Information

## 1.1 Lattice Boltzmann Method (LBM)

We employ a mesoscopic approach to simulate thermal convection in stabilised emulsions, by coupling a lattice Boltzmann method (LBM) [1, 2] for non-ideal multicomponent mixtures with a LBM for the temperature field dynamics. The model for multicomponent mixtures has been extensively used and analysed in previous works [3, 4, 5, 6, 7, 8, 9, 10]. Here we report its essential details. The emulsion is simulated with a two-component mixture (say $A$ and $B$). The associated LBM hinges on the dynamical evolution of mesoscopic probability density functions $f_\ell^i(\boldsymbol{x},t)$ of finding a particle of component $\ell = A,B$ in the space-time location $(\boldsymbol{x},t)$ with lattice velocity $\boldsymbol{c}^i$, where the index $i$ takes only a finite number of values. We employ a D2Q9 scheme (see Table 1), with 9 lattice velocities in a two-dimensional domain (i.e. $i = 0...8$) [1, 2]. The dynamical evolution of the distribution functions is ruled by the following discretised Boltzmann equation over a unitary time lapse $\Delta t = 1$

$$f_\ell^i(\boldsymbol{x}+\boldsymbol{c}^i,t+1) - f_\ell^i(\boldsymbol{x},t) = -\frac{1}{\tau}\left(f_\ell^i - f_\ell^{(eq,i)}\right)(\boldsymbol{x},t) + F_\ell^i(\boldsymbol{x},t). \tag{1}$$

Eq. (1) embeds a streaming step (l.h.s.) supplemented with local collisions (r.h.s.). The first term of the r.h.s. is the collision operator in the BGK approximation [11]; the term $F_\ell^i(\boldsymbol{x},t)$ is the source term [1, 2] and $\tau$ is a relaxation time towards the local equilibrium $f_\ell^{(eq,i)}$ (repeated indices are summed upon)

$$f_\ell^{(eq,i)} = w_i\rho_\ell\left[1 + \frac{u_k c_k^i}{c_s^2} + \frac{u_k u_p (c_k^i c_p^i - c_s^2\delta_{kp})}{2c_s^4}\right], \tag{2}$$

where $w_i$ are the usual D2Q9 weights [1, 2] and $c_s^2 = 1/3$ is the squared sound velocity (constant in the model). The density and global momentum fields

$$\rho_\ell(\boldsymbol{x},t) = \sum_i f_\ell^i(\boldsymbol{x},t) \tag{3}$$

$$\rho\boldsymbol{u}(\boldsymbol{x},t) = \sum_{\ell,i}\boldsymbol{c}^i f_\ell^i(\boldsymbol{x},t), \tag{4}$$

with $\rho = \sum_\ell \rho_\ell$, are coarse-grained fields suitably constructed from the distribution functions. The boundary conditions for the hydrodynamical fields correspond to a no-slip at the walls, which we achieve with the bounce-back rules [1, 2]. Periodic boundary conditions are applied in the $x$-direction.
The source term $F_\ell^i(\boldsymbol{x},t)$ includes the effects of interaction (int) forces, $\boldsymbol{F}_\ell^{\text{int}}(\boldsymbol{x},t)$, and external (ext) volume forces, $\boldsymbol{F}_\ell^{\text{ext}}(\boldsymbol{x},t)$. The first, in turn, includes three terms

$$\boldsymbol{F}_\ell^{\text{int}}(\boldsymbol{x},t) = \boldsymbol{F}_\ell^x(\boldsymbol{x},t) + \boldsymbol{F}_\ell^a(\boldsymbol{x},t) + \boldsymbol{F}_\ell^r(\boldsymbol{x},t). \tag{5}$$

The term $\boldsymbol{F}_\ell^x(\boldsymbol{x},t)$ is a phase-segregating interaction between the two components. It is introduced in the model to promote the formation of stable interfaces separating bulk regions with the majority of one of the two components. This phase-segregating interaction is implemented following the Shan-Chen model [12] for multicomponent mixtures:

$$\boldsymbol{F}_\ell^x(\boldsymbol{x},t) = -\frac{\mathscr{G}_{AB}}{\rho_0^2}\rho_\ell(\boldsymbol{x},t)\sum_{\ell',\ell'\neq\ell}\sum_{i\in NN} w_i\rho_{\ell'}(\boldsymbol{x}+\boldsymbol{c}^i,t)\boldsymbol{c}^i \tag{6}$$

where $\rho_0$ is a reference density and $\mathscr{G}_{AB}$ is a positive coupling constant between species dictating the strength of phase segregating interactions. The set $NN$ refers to the set of nearest neighbours of point $\boldsymbol{x}$ on the lattice: this set coincides with the set of the D2Q9 directions used for the streaming of the LBM populations (see table 1). The two contributions $\boldsymbol{F}_\ell^a(\boldsymbol{x},t)$ and $\boldsymbol{F}_\ell^r(\boldsymbol{x},t)$ represent competing interactions [3], i.e. short-range attractive ($a$) and long-range repulsive ($r$) interactions. They are introduced at the interface to inhibit the coalescence of droplets. Mechanically, they introduce a positive disjoining pressure [4]. In formulae, they read [7]:

$$\boldsymbol{F}_\ell^a(\boldsymbol{x},t) = -\mathscr{G}_{\ell\ell}^a\psi_\ell(\boldsymbol{x},t)\sum_{i\in NN} w_i\psi_\ell(\boldsymbol{x}+\boldsymbol{c}^i,t)\boldsymbol{c}^i \tag{7}$$

$$\boldsymbol{F}_\ell^r(\boldsymbol{x},t) = -\mathscr{G}_{\ell\ell}^r\psi_\ell(\boldsymbol{x},t)\left[\sum_{i\in NN} p_i\psi_\ell(\boldsymbol{x}+\boldsymbol{c}^i,t)\boldsymbol{c}^i + \sum_{i\in NNN} p_i\psi_\ell(\boldsymbol{x}+\boldsymbol{c}^i,t)\boldsymbol{c}^i\right], \tag{8}$$

| $w_i = w(\boldsymbol{c}^i)$ | $p_i = p(\boldsymbol{c}^i)$ | $\lvert\boldsymbol{c}^i\rvert$ | $\boldsymbol{c}^i$ | $i$ |
|---|---|---|---|---|
| 4/9 | 247/420 | 0 | (0,0) | 0 |
| 1/9 | 4/63 | 1 | $(\pm1,0);(0,\pm1)$ | 1-4 |
| 1/36 | 4/135 | 2 | $(\pm1,\pm1)$ | 5-8 |
| 0 | 1/180 | 4 | $(\pm2,0)$ ; $(0,\pm2)$ | 9-12 |
| 0 | 2/942 | 5 | $(\pm1,\pm2)$; $(\pm2;\pm1)$ | 13-20 |
| 0 | 1/15120 | 8 | $(\pm2,\pm2)$ | 21-24 |

Table 1: Weights list of Eq. (6), (7) and (8). The set of nearest neighbours (NN) is referred to index $i = 0...8$, while next-nearest neighbours (NNN) are links with index $i = 9...24$.

with $\mathscr{G}^a_{\ell\ell} < 0$, $\mathscr{G}^r_{\ell\ell} > 0$. In the above expressions, $\psi_\ell(\boldsymbol{x},t) = \psi(\rho_\ell(\boldsymbol{x},t))$ is the *pseudo-potential* of the Shan-Chen formulation for multiphase systems [12]:

$$\psi_\ell(\boldsymbol{x},t) = \rho_0\left[1 - \exp(-\rho_\ell(\boldsymbol{x},t)/\rho_0)\right]. \tag{9}$$

The set *NNN* in (8) refers to next-to-nearest neighbours, i.e. an additional layer of 16 lattice velocities. The numerical values of the weights are detailed in Table 1. The numerical simulations described in the main paper use $\rho_0 = 0.83$, $\mathscr{G}_{AB} = 0.405$, $\mathscr{G}^a_{AA} = -9.0$, $\mathscr{G}^a_{BB} = -8.0$, $\mathscr{G}^r_{AA} = 8.1$, $\mathscr{G}^r_{BB} = 7.1$, all values given in lattice Boltzmann units (lbu). Regarding the external volume forces $\boldsymbol{F}^{\text{ext}}_\ell(\boldsymbol{x},t)$, a buoyancy term is added to the global momentum balance in the Boussinesq's form

$$\boldsymbol{F}^{\text{ext}}_\ell(\boldsymbol{x},t) = \rho_\ell(\boldsymbol{x},t)\,\alpha\, g\, T(\boldsymbol{x},t)\,\boldsymbol{e}_y, \tag{10}$$

where $T(\boldsymbol{x},t)$ is the temperature field relative to some reference temperature, $\alpha$ the thermal expansion coefficient, $g$ the gravity acceleration and $\boldsymbol{e}_y$ the unit vector in the wall-to-wall direction. By summing over the components $\ell$, one can construct the total force

$$\boldsymbol{F}(\boldsymbol{x},t) = \sum_\ell \mathbf{F}_\ell = \sum_\ell \boldsymbol{F}^{\text{int}}_\ell(\boldsymbol{x},t) + \sum_\ell \boldsymbol{F}^{\text{ext}}_\ell(\boldsymbol{x},t) = \boldsymbol{F}^{\text{int}}(\boldsymbol{x},t) + \boldsymbol{F}^{\text{ext}}(\boldsymbol{x},t). \tag{11}$$

At large scales, the long wavelength limit of the lattice Boltzmann model maps into the diffuse-interface Navier-Stokes-Boussinesq equations [1, 2]:

$$\rho\left(\partial_t + u^{(\mathrm{H})}_k\partial_k\right)u^{(\mathrm{H})}_i = -\partial_j P_{ij} + \eta_0\partial_j\left(\partial_i u^{(\mathrm{H})}_j + \partial_j u^{(\mathrm{H})}_i\right) + \rho\alpha g T\delta_{iy} \qquad i = x,y \tag{12}$$

where $\rho\boldsymbol{u}^{(\mathrm{H})} = \rho\boldsymbol{u} + \boldsymbol{F}^{\text{int}}/2 + \boldsymbol{F}^{\text{ext}}/2$ is the hydrodynamical momentum of the mixture. The non-ideal pressure tensor $P_{ij}$ is non-diagonal due to the contribution of interaction forces [13, 14]. The precise expression of $P_{ij}$ can be written starting from the knowledge of the interaction forces. Details on the calculations can be found in [8]. It is important to stress that the bulk viscosity $\eta_0$ is linked to the relaxation time $\tau$ of the lattice Boltzmann equation (1) according to the following relation [1, 2]:

$$\eta_0 = \rho c_s^2\left(\tau - \frac{1}{2}\right). \tag{13}$$

Hence, $\eta_0$ can be tuned via a proper choice of the relaxation time in the lattice Boltzmann dynamics (1). The evolution of the temperature field $T(\boldsymbol{x},t)$ is integrated via another properly devised lattice Boltzmann scheme [15]. In a nutshell, we evolve in time an auxiliary probability distribution function $g^i(\boldsymbol{x},t)$, whose coarse-grained counterpart is the temperature field:

$$T(\boldsymbol{x},t) = \sum_i g^i(\boldsymbol{x},t). \tag{14}$$

This is a popular strategy used in the LBM frameworks [1, 2] that we briefly recall here. The mesoscopic dynamics for $g^i(\boldsymbol{x},t)$ reads as follow:

$$g^i(\boldsymbol{x}+\boldsymbol{c}^i,t+1) - g^i(\boldsymbol{x},t) = -\frac{1}{\tau_g}\left(g^i - g^{(eq,i)}\right)(\boldsymbol{x},t), \tag{15}$$

where the local equilibrium $g^{(eq,i)}$ takes now the form

$$g^{(eq,i)} = w_i T\left[1 + \frac{u^{(\mathrm{H})}_k c^i_k}{c_s^2} + \frac{u^{(\mathrm{H})}_k u^{(\mathrm{H})}_p (c^i_k c^i_p - c_s^2\delta_{kp})}{2c_s^4}\right].$$

The long-wavelength limit of (15) approximates the advection-diffusion equation for the temperature field

$$\partial_t T + u_k^{(\mathrm{H})} \partial_k T = \kappa \partial_{kk} T \tag{16}$$

where

$$\kappa = c_s^2 \left( \tau_g - \frac{1}{2} \right) \tag{17}$$

is the *thermal diffusivity* which can be tuned by changing the thermal relaxation time $\tau_g$. The advection-diffusion equation (16) is two-way coupled with the Navier-Stokes equations (12) via i) the fluid velocity field entering the advection term in (16) and ii) the buoyancy force in the r.h.s. of (12).

## 1.2 Time-Averaged Nusselt Number: effective modelling at the droplet scale

In Fig. 1 we report the behaviour of the time-averaged Nusselt number $\langle \mathrm{Nu} \rangle_t$ as a function of the droplet concentration $\Phi_0$ together with the Nusselt number obtained from single-phase (SP) simulations with 2 different choices for the viscosity of the SP system, based on Eq. (5) (brown triangles) and (6) (diamond-shaped blue points) of the main paper. This figure highlights that the time-average of the Nusselt number of the emulsions stays in between these two estimates.
Fig. 2 shows the viscosity profiles as a result of the coarse-graining procedure on $\eta_\Lambda^{\mathrm{SP}}(y)$ (cfr. Eq. (7) of the main paper) for $\Lambda = 0, 3d$ and $\Lambda \to \infty$ (the latter corresponding to a constant effective viscosity) and for different values of $\Phi_0$. The values of $\eta_{\mathrm{rheo}}^{\mathrm{SP}}(\Phi_0)$ are also reported for comparison.

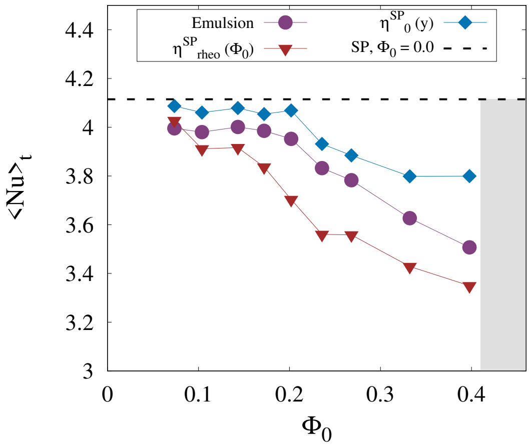


Figure 1: We report data given in Fig. 6 in the main paper with the additional curve of the Nusselt number for a single-phase (SP) system with a local viscosity $\eta_0^{\mathrm{SP}}(y)$ given by Eq. (6) of the main paper. The dark region refers to a range of concentrations for which non-Newtonian effects start to emerge (cfr. Fig. 2 in the main paper).

## 1.3 Anomalous heat transfer fluctuations: from large scales to the droplet scale

In Fig. 3 we report the rheological characterisation of both Newtonian (NE) and non-Newtonian (NNE) emulsions that are used to obtain the results discussed in Section 6 of the main paper. Both emulsions are confined in a channel with width $H/d = 25$, with $d$ the mean droplet diameter. In panel (a) we report the flow curves relating the stress $\Sigma$ to the shear rate $\dot{\gamma}$, obtained with dedicated shear experiments (see the main paper for details). In panel (b) we report the effective dynamic viscosity $\eta_{\mathrm{eff}}(\dot{\gamma}) = \mathrm{d}\Sigma(\dot{\gamma})/\mathrm{d}\dot{\gamma}$ as a function of the shear rate $\dot{\gamma}$ extracted from the flow curves in panel (a).

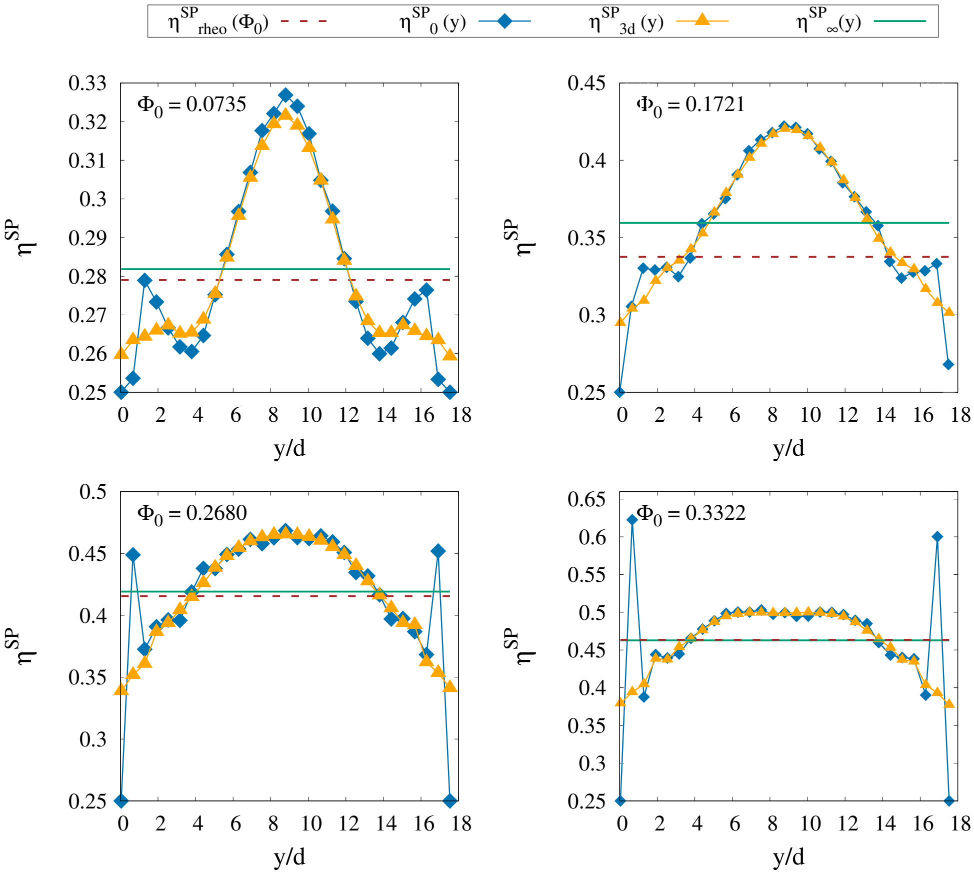


Figure 2: Viscosity profiles $\eta^{\mathrm{SP}}(y)$ for different concentrations $\Phi_0$ of the emulsions. Predictions for $\eta^{\mathrm{SP}}_{\mathrm{rheo}}(\Phi_0)$ from protocol given in Eq. (5) of the main paper are compared with predictions $\eta^{\mathrm{SP}}_{\Lambda}(y)$ from protocol given in Eq. (7) of the main paper using various resolutions of the coarse-graining parameter $\Lambda$ (cfr. Eq. (8) of the main paper). The $y$-coordinate is normalised by the mean droplet diameter $d$. Viscosities are reported lattice Boltzmann simulation units.

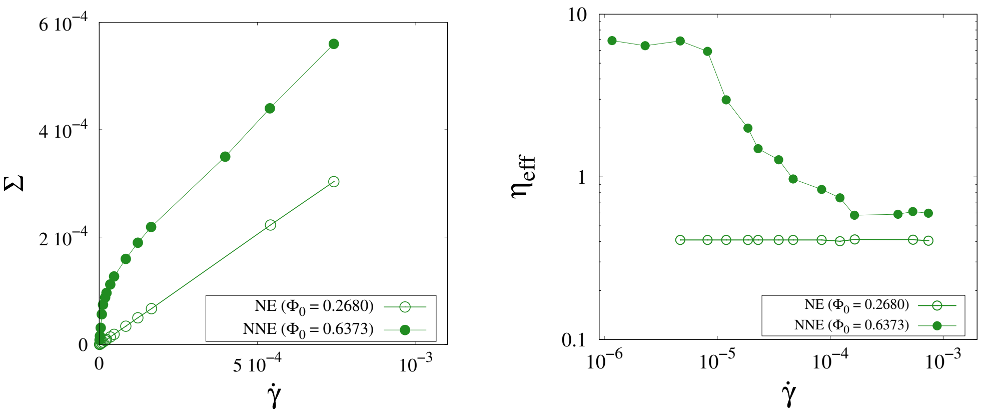


(a) (b)

Figure 3: Shear rheological characterisation of both NE and NNE discussed in Section 6 of the main paper. Panel (a): flow curves. Panel (b): the extracted emulsion effective viscosity $\eta_{\mathrm{eff}}(\dot{\gamma}) = \mathrm{d}\Sigma(\dot{\gamma})/\mathrm{d}\dot{\gamma}$. A movie of both NE and NNE is included in this ESI. All dimensional quantities are reported in lattice Boltzmann units.

# References


[1] S. Succi, *The lattice Boltzmann Equation*, Oxford University Press, 2018.

[2] T. Krüger, H. Kusumaatmaja, A. Kuzmin, O. Shardt, G. Silva and E. M. Viggen, *Springer International Publishing*, 2017, **10**, 4–15.

[3] R. Benzi, M. Sbragaglia, S. Succi, M. Bernaschi and S. Chibbaro, *J. Chem. Phys.*, 2009, **131**,.

[4] M. Sbragaglia, R. Benzi, M. Bernaschi and S. Succi, *Soft Matter*, 2012, **8**, 10773–10782.

[5] R. Benzi, M. Bernaschi, M. Sbragaglia and S. Succi, *Europhys. Lett.*, 2013, **104**, 48006.

[6] R. Benzi, M. Sbragaglia, P. Perlekar, M. Bernaschi, S. Succi and F. Toschi, *Soft Matter*, 2014, **10**, 4615–4624.

[7] R. Benzi, M. Sbragaglia, A. Scagliarini, P. Perlekar, M. Bernaschi, S. Succi and F. Toschi, *Soft Matter*, 2015, **11**, 1271–1280.

[8] B. Dollet, A. Scagliarini and M. Sbragaglia, *J. Fluid Mech.*, 2015, **766**, 556–589.

[9] L. Fei, A. Scagliarini, A. Montessori, M. Lauricella, S. Succi and K. H. Luo, *Physical Review Fluids*, 2018, **3**, 104304.

[10] F. Pelusi, M. Sbragaglia and R. Benzi, *Soft Matter*, 2019, **15**, 4518–4524.

[11] P. L. Bhatnagar, E. P. Gross and M. Krook, *Physical review*, 1954, **94**, 511.

[12] X. Shan and H. Chen, *Physical Review E*, 1993, **47**, 1815.

[13] X. Shan, *Physical Review E*, 2008, **77**, 066702.

[14] M. Sbragaglia and D. Belardinelli, *Physical Review E*, 2013, **88**, 013306.

[15] P. Ripesi, L. Biferale, M. Sbragaglia and A. Wirth, *Journal of fluid mechanics*, 2014, **742**, 636–663.
